# Supplementary material for: Motion Perceiver: Real-Time Occupancy Forecasting for Embedded Systems
Source: arXiv:2306.08879 source file (2024-02-02)
Supplement: Supplementary file 1 [file appendix.tex]

\newpage

\section{Appendix}

\subsection{Occlusion in Waymo Open Motion Dataset}

The Waymo Open Motion Dataset (WOMD) is captured on Waymo's self driving car platform. This results significant occlusions in tracked agent trajectories, and the occasional ID switch. This is particularly problematic towards the end of the sequence where approximately half of the agents observed in the past and current frames are unobserveable in the future frames, shown in Fig. \ref{fig:waymo_tracked}. 

\begin{figure}[hbt]
    \centering
    \includegraphics[width=3.2in]{misc/waymo_agent_decay.png}
    \caption{The percentage of observable agents that are present in each frame diminish over time as they are occluded from the view of the self driving car.}
    \label{fig:waymo_tracked}
\end{figure}

This results in an overestimation of the false positive rate due to poor ground truth data. This is shown in Fig. \ref{fig:waymo_fut_occ} where the model correctly predicts an occluded vehicle's position in future frames, but it is missing from the ground truth. Datasets such as Interaction \cite{Interaction} are collected from a fixed position at a point of interest, resulting in consistent observability of the map over time.

\begin{figure}[hbt]
    \centering
    \begin{tabular}{c c c}
        \subfloat[0s]{\includegraphics[width=0.95in]{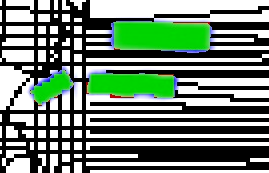}} &
        \subfloat[3s]{\includegraphics[width=0.95in]{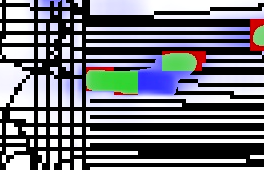}} &
        \subfloat[3.7s]{\includegraphics[width=0.95in]{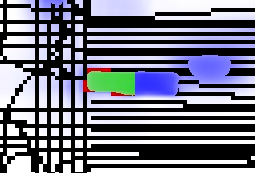}} \\
    \end{tabular}
    \caption{The evaluated false positive rate is overestimated as vehicles are frequently occluded in the ground truth. Two of the three cars observed in the current frame (a) are lost in future frames, shown in (b) and (c), resulting in a false positive prediction shown in blue. }
    \label{fig:waymo_fut_occ}
\end{figure}

\subsection{Speculative Prediction}

The future frames of Waymo Open Motion includes detections of agents that have not been observed in past or present frames, which the dataset categorizes as occluded vehicles. We found that care needs to be taken to filter out these unobserved agents. The speculative prediction that arises from the inclusion of occluded agents in the ground truth loss hinders statistical performance, Table \ref{tab:observ_filt}. An example of speculative prediction where no ground truth occluded agents appear is shown in Fig. \ref{fig:speculation}. Furthermore, there are areas where a homogeneous cloud of occupancy grows (Fig. \ref{fig:occ_cloud}). This speculative prediction is removed by only training models to predict occupancy for observable agents, as shown in Table \ref{tab:observ_filt}.

% Training with unfiltered data results in a growing homogeneous low probability cloud as the network tries to speculate about agents which appear in the future, shown by the background noise in in Fig. \ref{fig:speculation}. Inclusion of these future agents pollutes the loss function and distracts from learning to predict the motion of agents which have actually been observed up to a given time step.

\begin{figure}[hbt]
    \centering
    \begin{tabular}{ c c }
    \subfloat[+0s]{\includegraphics[width=1.5in]{speculation/speculate_t+0.png}} &
    \subfloat[+1s]{\includegraphics[width=1.5in]{speculation/speculate_t+10.png}} \\
    \subfloat[+2s]{\includegraphics[width=1.5in]{speculation/speculate_t+20.png}} &
    \subfloat[+4s]{\includegraphics[width=1.5in]{speculation/speculate_t+40.png}} \\
    \end{tabular}
    \caption{ \networkName{} speculatively predicts occupancy when training on ground truth data that includes the occupancy of previously occluded agents observed in the future. However this has an overall detrimental effect on statistical performance, shown in Table \ref{tab:observ_filt}. }
    \label{fig:speculation}
\end{figure}

\begin{figure}[hbt]
    \centering
    \begin{tabular}{ c c }
    \subfloat[+0s]{\includegraphics[width=1.5in]{occ_cloud/occ_cloud_+0s.png}} &
    \subfloat[+1s]{\includegraphics[width=1.5in]{occ_cloud/occ_cloud_+3s.png}} \\
    \end{tabular}
    \caption{Speculative occupancy is predicted in areas around parked cars. This can be attributed to the common behaviour of parked cars becoming un-occluded in the future as the data collection vehicle passes them.}
    \label{fig:occ_cloud}
\end{figure}

\begin{table}[hbt]
    \centering
    \begin{tabular}{|c|c|c|c|}
        \hline
        \textbf{Ground} & \multicolumn{3}{|c|}{\textbf{IoU}}            \\
        \textbf{Truth}  & \textbf{+0s}  & \textbf{+3s}  & \textbf{+6s}  \\
        \hline
        % eee79137f83652567e426d86eed7d637
        All             & 0.8555        & 0.4875        & 0.3280        \\
        % 6e5c186e7772327882dcc8840d1ee6a4
        Observable      & \textbf{0.890}& \textbf{0.511}& \textbf{0.351}\\ 
        \hline
    \end{tabular}
    \caption{Statistical performance increases when only training to predict occupancy of observable agents.}
    \label{tab:observ_filt}
\end{table}

\subsection{Class Aware Occupancy}

We briefly evaluate class-aware occupancy by using a separate MLP decoder for each class when querying occupancy (refer to eq. \ref{eq:outputQuery} and \ref{eq:tformer}). We remind the reader that the input to the model already includes a one-hot encoding of the agent class. Cyclists are not reported by other methods, but also performs worse than pedestrians for our method (SoftIoU $<$ 0.02), indicating that this is an under-represented class requiring substantially more investigation in future research.

\begin{table}[hbt]
    \centering
    \begin{tabular}{|c|c|c|c|c|c|}
        \hline
        \textbf{Waymo @ 3s}             & \multicolumn{2}{|c|}{Pedestrians} & \multicolumn{2}{|c|}{Vehicles}    \\
        \textbf{Future}                 & \textbf{Soft IoU} & \textbf{AUC}  & \textbf{Soft IoU} & \textbf{AUC}  \\
        \hline
        STOPNet \cite{STOPNet}          & \textbf{0.27}     & 0.59          & \textbf{0.53}     & 0.86          \\
        FlowFields \cite{OccupancyFlow} & 0.25              & 0.5           & 0.52              & 0.84          \\
        % e4775c11ba53b9fdcbf1aab379e4a504
        Ours*                           & 0.12              & \textbf{0.92} & \textbf{0.53}     & \textbf{0.98} \\ 
        \hline
    \end{tabular}
    \caption{
        Performance comparison with other occupancy prediction models on WOMD at $3s$ into the future with class sensitive output. These results are not directly comparable, as it is unclear what dataset the baseline results were captured on. * denotes that we use our evaluation method in our chosen reference frame using the scenarios from WOMD validation set evaluation server.
    }
    \label{tab:waymo_cls_perf}
\end{table}

\subsection{Learnt Social Interactions}

We include interesting social dynamics learnt by \networkName{} (Fig. \ref{fig:socialDynMerge}, \ref{fig:socialDynStop}, \ref{fig:socialDynStart}), these scenarios are also included in the supplementary video. We show in the top right the time frame index of the sequence, relative to the present frame i.e. ``future: +80" is 8sec into the future.

\begin{figure}[hbt]
    \centering
    \begin{tabular}{c c c}
         \subfloat[+0s]{\includegraphics[width=0.7in]{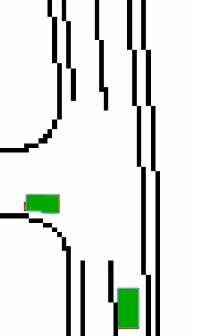 }} &
         \subfloat[+2s]{\includegraphics[width=0.7in]{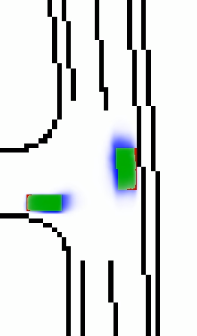}} &
         \subfloat[+4s]{\includegraphics[width=0.7in]{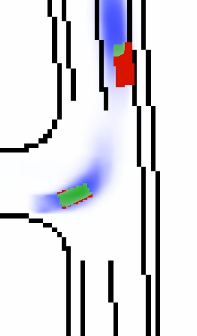}} \\
    \end{tabular}
    \caption{The sequence above demonstrates \networkName{}'s ability to predict motion based off social dynamics and is from the same sequence as Fig. \ref{fig:socialDynMergeNoCtx}, but we now have road-graph topology and traffic signal context.}
    \label{fig:socialDynMerge}
\end{figure}

\begin{figure}[hbt]
    \centering
    \begin{tabular}{c c}
         \subfloat{\includegraphics[width=1.5in]{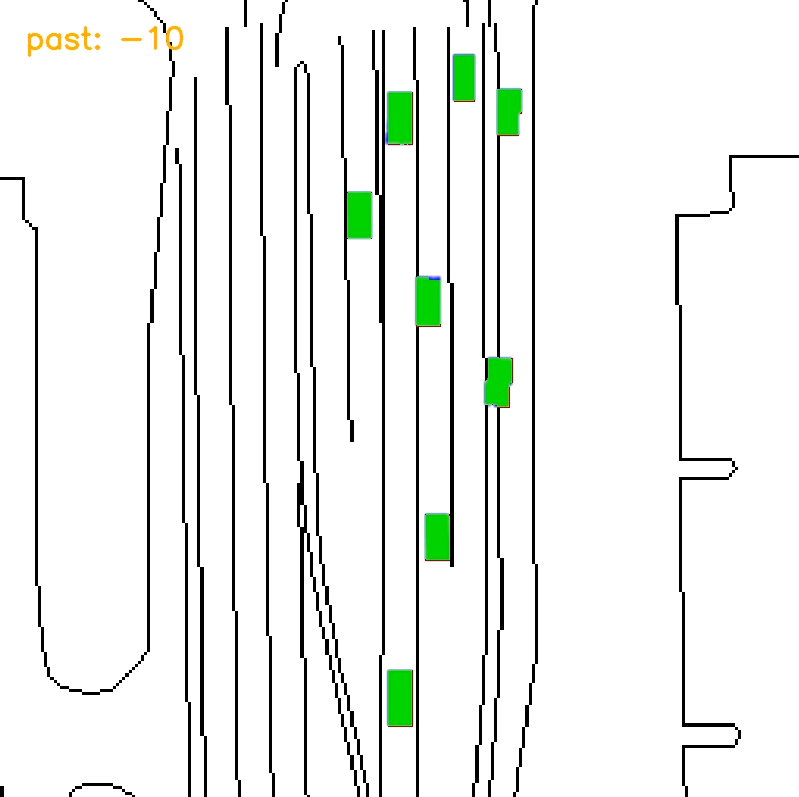}} &
         \subfloat{\includegraphics[width=1.5in]{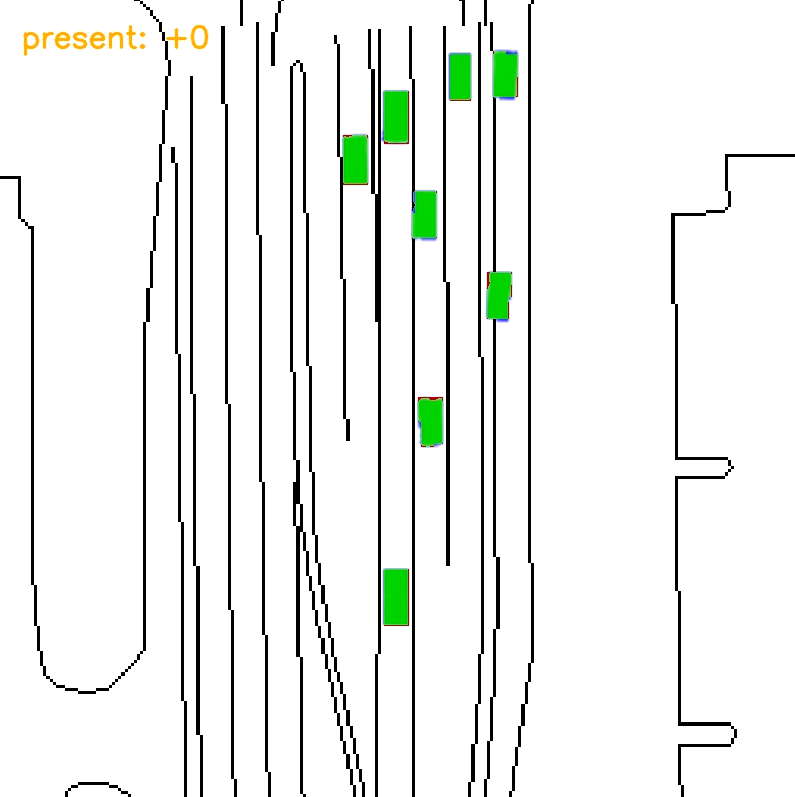 }} \\
         \subfloat{\includegraphics[width=1.5in]{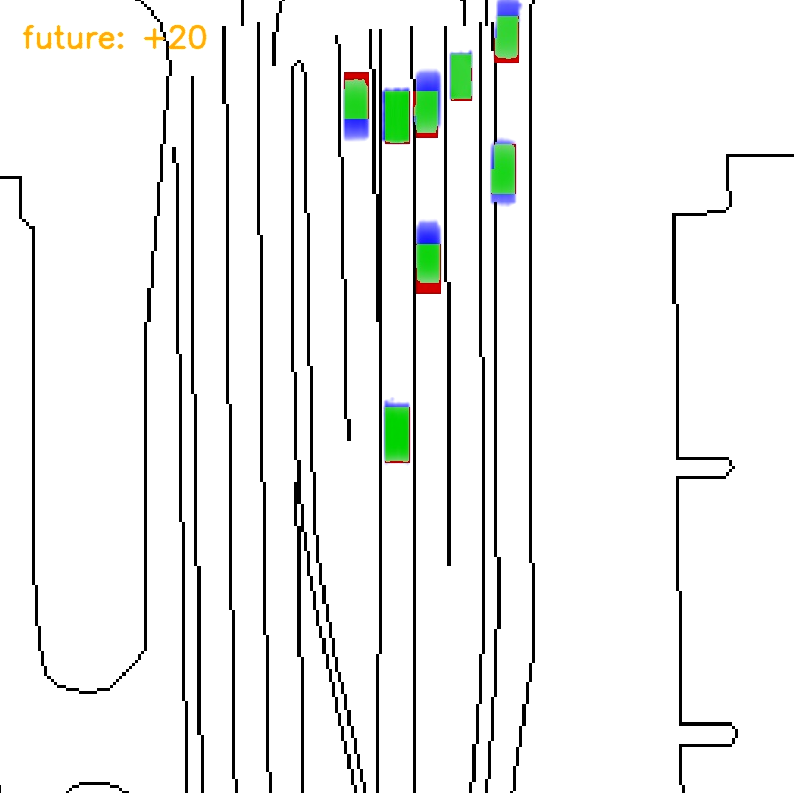}} &
         \subfloat{\includegraphics[width=1.5in]{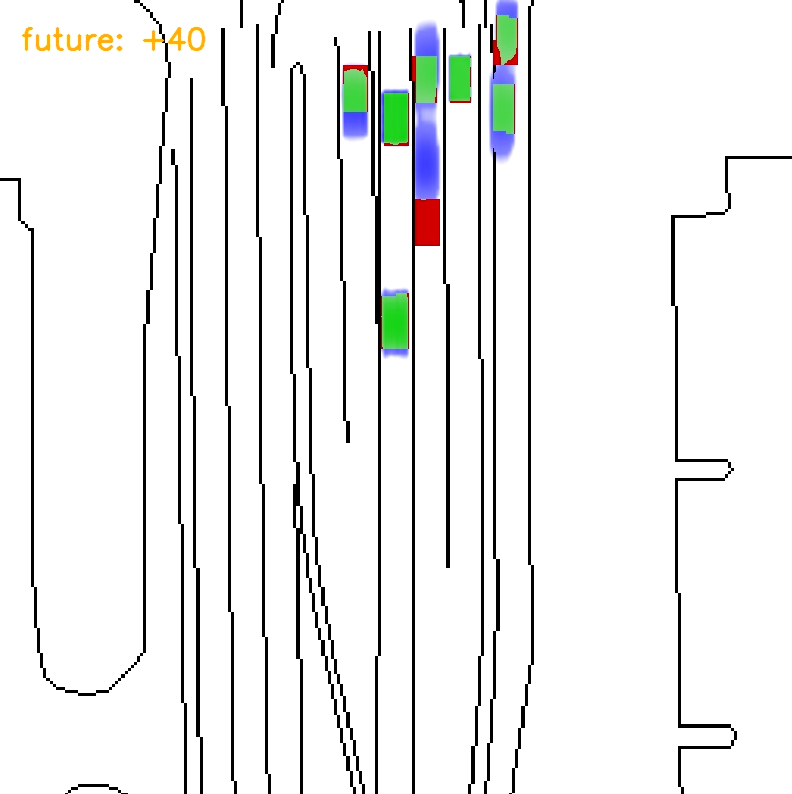}} \\
         \subfloat{\includegraphics[width=1.5in]{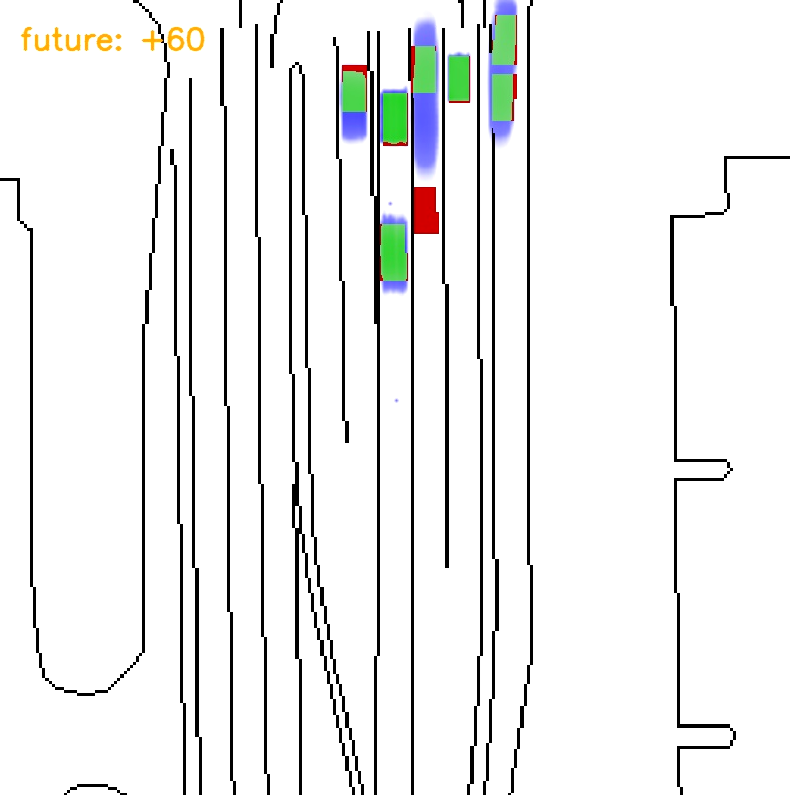}} &
         \subfloat{\includegraphics[width=1.5in]{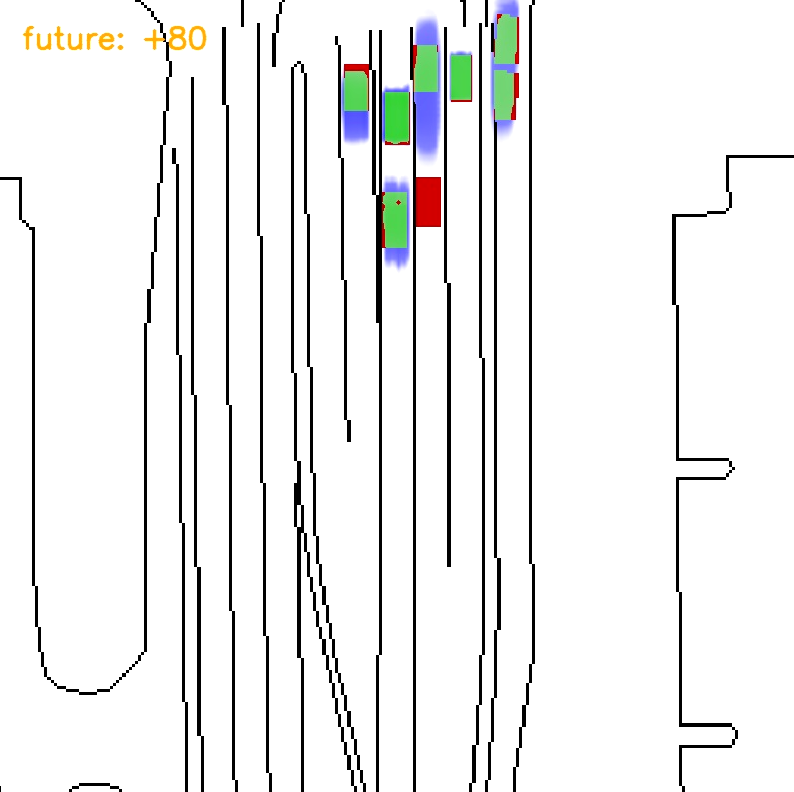}} \\
    \end{tabular}
    \caption{This sequence demonstrates cars approaching an intersection (presumably at a stop light). The occupancy at the end of the sequence shows a prediction of all vehicles coming to a stop. The major source of error in this prediction is the unexpected behaviour of the vehicle in the middle which stopped significantly behind of the car in-front, rather than queuing closely like others.}
    \label{fig:socialDynStop}
\end{figure}

\begin{figure}[hbt]
    \centering
    \begin{tabular}{c c}
         \subfloat{\includegraphics[width=1.5in]{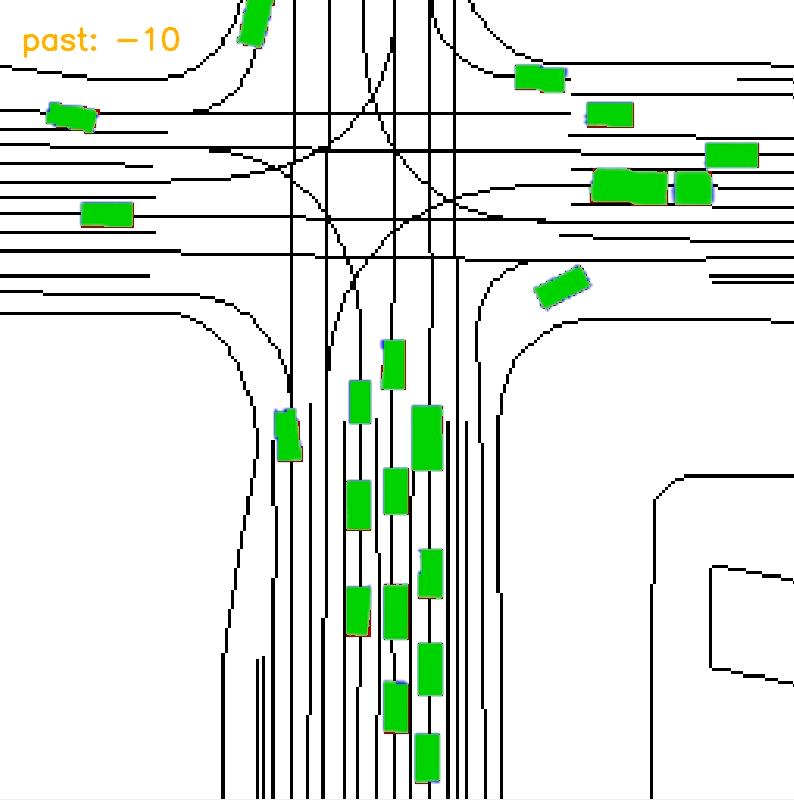}} &
         \subfloat{\includegraphics[width=1.5in]{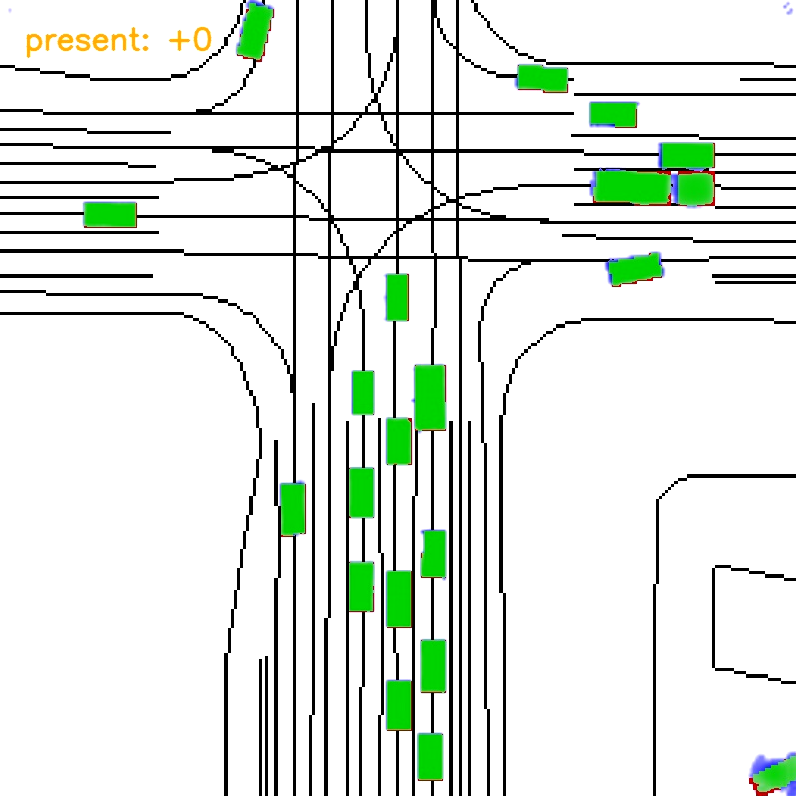 }} \\
         \subfloat{\includegraphics[width=1.5in]{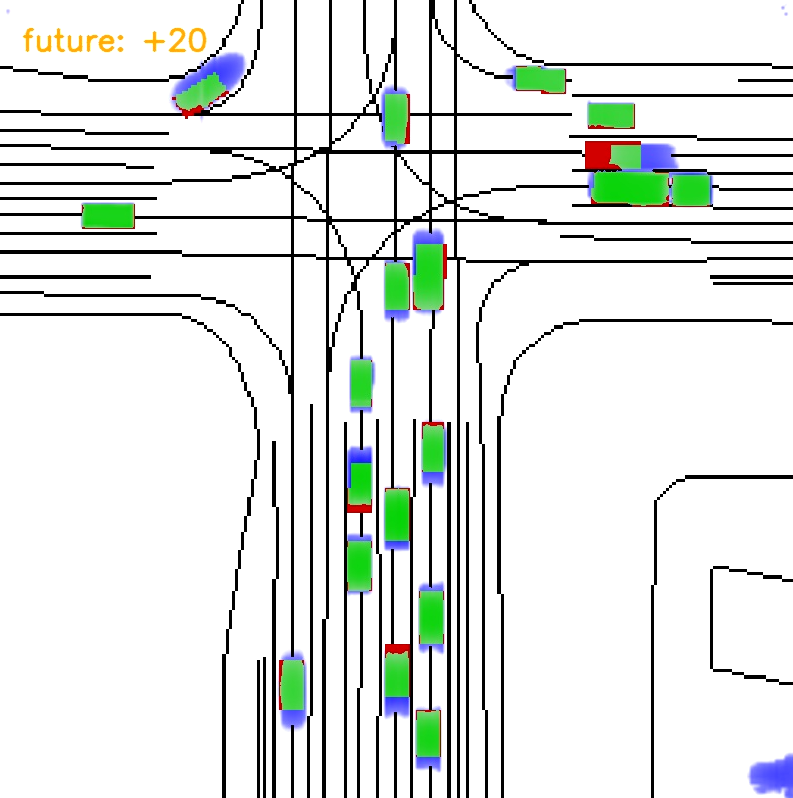}} &
         \subfloat{\includegraphics[width=1.5in]{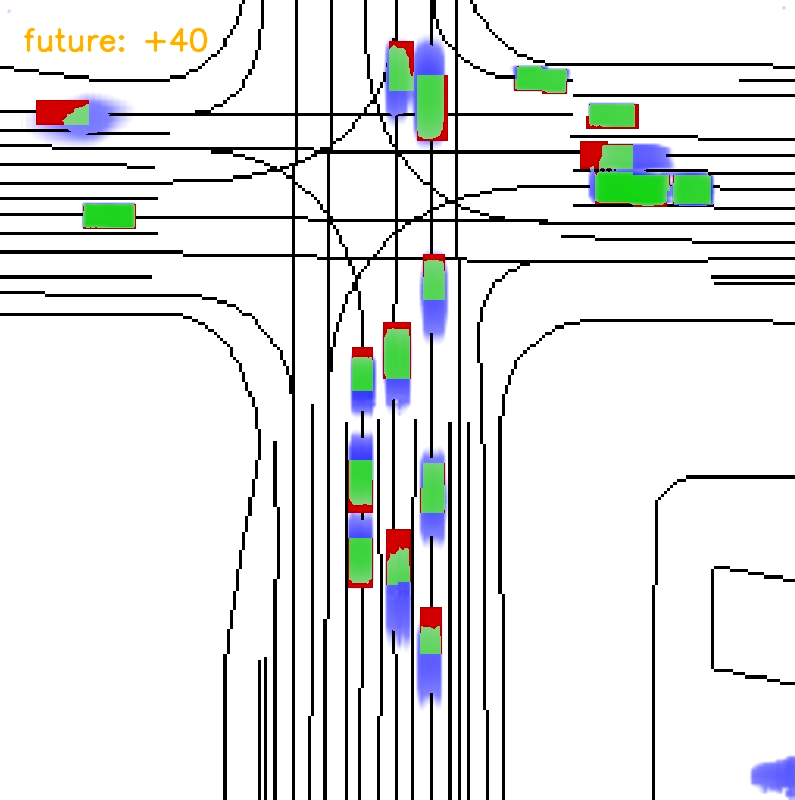}} \\
         \subfloat{\includegraphics[width=1.5in]{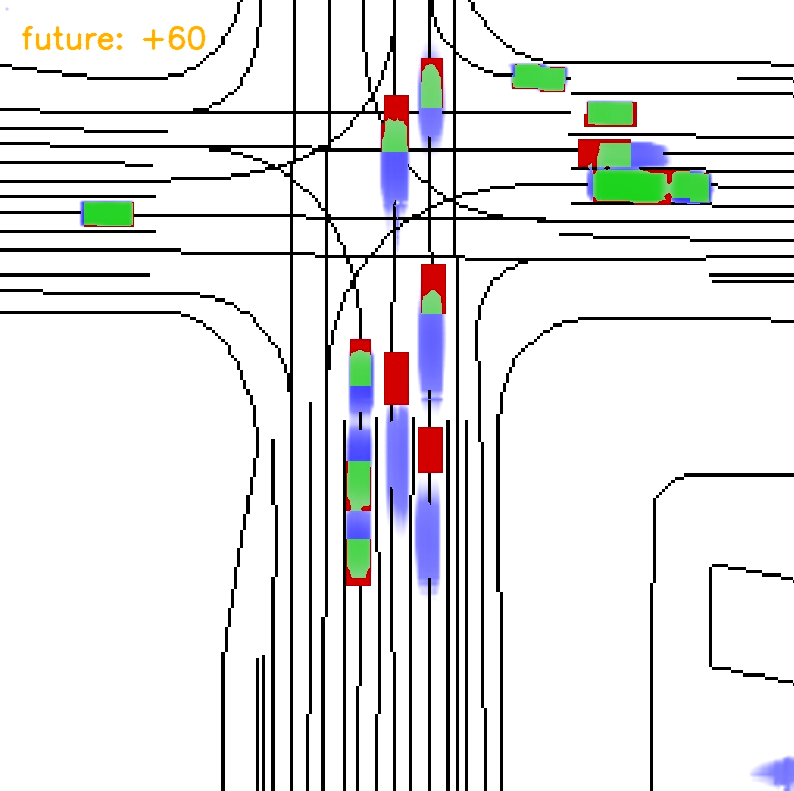}} &
         \subfloat{\includegraphics[width=1.5in]{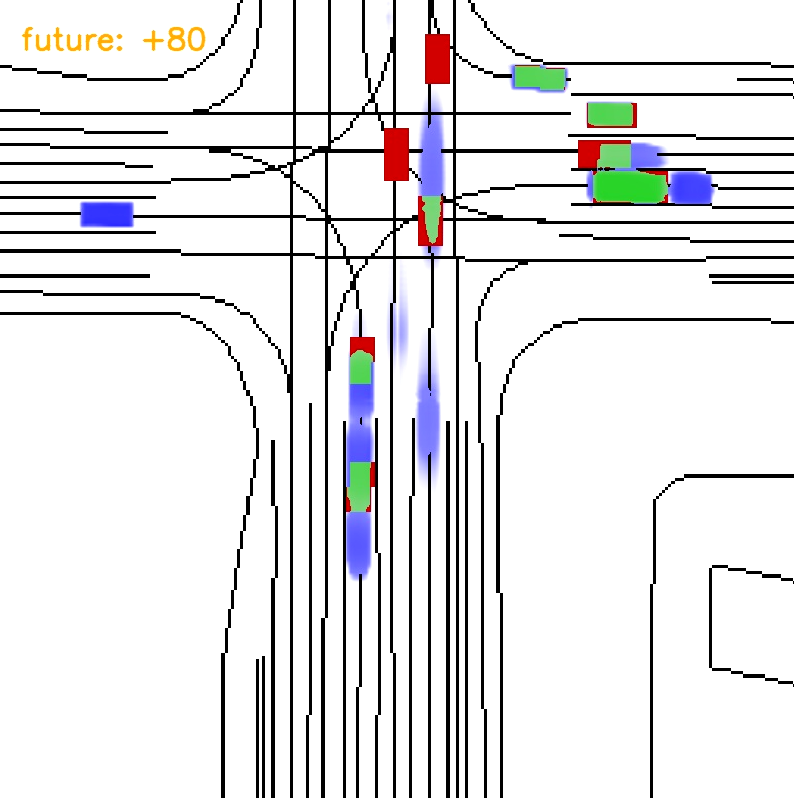}} \\
    \end{tabular}
    \caption{The scenario above shows vehicles accelerating from a traffic light that has recently transitioned green. \networkName{} correctly predicts the acceleration of the first rows before the last rows. However the rate of acceleration is underestimated, causing the forecast occupancy to trail behind the ground truth vehicles.}
    \label{fig:socialDynStart}
\end{figure}

\subsection{Model Architecture}

The parameters used for the model with all context available are shown in Table \ref{tab:network_params}. We note that we add a dummy agent and signal feature because if there is no measured agents/signals and the entire input is masked, PyTorch's Transformer output is NaN. This is a constant dummy token of all zeros.

\begin{table}[hbt]
    \centering
    \begin{tabular}{|c|c|c|}
        \hline
        \textbf{Module}         & \textbf{Parameter}    & \textbf{Value}    \\
        \hline
        \multicolumn{3}{|c|}{\textbf{Latent State}}                         \\
        \hline
                                & num variables         & 128               \\
                                & num channels          & 256               \\
        \hline
        \multicolumn{3}{|c|}{\textbf{Initialisation Layer}}                 \\
        \hline
        Cross-Attention Layer   & q channels            & 256               \\
                                & kv channels           & 392               \\
                                & num heads             & 4                 \\
        Self-Attention Block    & num layers            & 6                 \\
                                & qkv channels          & 256               \\
                                & num heads             & 4                 \\
        \hline
        \multicolumn{3}{|c|}{\textbf{Time Evolution Layer}}                 \\
        \hline
        Self-Attention Block    & num layers            & 6                 \\
                                & qkv channels          & 256               \\
                                & num heads             & 4                 \\
        \hline
        \multicolumn{3}{|c|}{\textbf{Agent Encoder}}                        \\
        \hline
        Feature Encoder         & num pos frequencies   & 64                \\
                                & num yaw frequencies   & 16                \\
                                & max frequency         & 200               \\
                                & max tokens            & 128+1             \\
                                & \textbf{out channels} & 64*2*3+5+3        \\
        \hline
        \multicolumn{3}{|c|}{\textbf{Agent Update Layer}}                   \\
        \hline
        Cross-Attention Layer   & q channels            & 256               \\
                                & kv channels           & 392               \\
                                & num heads             & 4                 \\
        \hline
        \multicolumn{3}{|c|}{\textbf{Signal Encoder}}                       \\
        \hline
        Feature Encoder         & num pos frequencies   & 30                \\
                                & max frequency         & 200               \\
                                & max tokens            & 16+1              \\
                                & \textbf{out channels} & 30*2*2+8          \\
        Self-Attention Layer    & qkv channels          & 256               \\
                                & num heads             & 4                 \\
        \hline
        \multicolumn{3}{|c|}{\textbf{Signal Update Layer}}                  \\
        \hline
        Cross-Attention Layer   & q channels            & 256               \\
                                & kv channels           & 128               \\
                                & num heads             & 4                 \\
        \hline
        \multicolumn{3}{|c|}{\textbf{Road Topology Encoder}}                \\
        \hline
        Feature Encoder         & raster resolution     & 256               \\
                                & patch resolution      & 32                \\
                                & num pos frequencies   & 16                \\
                                & mlp feature enc       & 190               \\
                                & \textbf{out channels} & 190+66            \\
        \hline
        \multicolumn{3}{|c|}{\textbf{Road Topology Update Layer}}           \\
        \hline
        Cross-Attention Layer   & q channels            & 128               \\
                                & kv channels           & 256               \\
                                & num heads             & 4                 \\
        Self-Attention Layer    & qkv channels          & 256               \\
                                & num heads             & 4                 \\
        \hline
        \multicolumn{3}{|c|}{\textbf{Occupancy Query Token}}                \\
        \hline
        Feature Encoder         & num pos frequencies   & 32                \\
                                & max frequency         & 256               \\
                                & image resolution      & 256               \\
        \hline
        \multicolumn{3}{|c|}{\textbf{Output Decoder}}                       \\
        \hline
        Cross-Attention Layer   & q channels            & 6                 \\
                                & kv channels           & 256               \\
                                & num heads             & 4                 \\
                                & residual connection   & False             \\
        Output MLP              & input channels        & 256               \\
                                & output channels       & 1                 \\
        \hline
    \end{tabular}
    \caption{We list our models modules and their dimensionality. MLP layer applied after multi-Head attention are of same channels as the query input and are omitted for brevity.}
    \label{tab:network_params}
\end{table}
